# Supplementary material for: Contention resolution on a restrained channel
Source: arXiv:1808.02216 source file (2020-05-16)
Supplement: Supplementary file 1 [file appendix.tex]

\textbf{\large Supplemental Materials: \\ Energy Aware Parallel Queuing \\ With Contention}
\setcounter{equation}{0}
\setcounter{figure}{0}
\setcounter{table}{0}
\setcounter{page}{1}
\setcounter{section}{1}

\subsection{Model relevance for \algoname{Backoff} protocol}
In general we follow the model from \cite{hastad}. That is, we do not terminate undelivered messages, we have a message length limited to the length of the transmission phase in a single round, and we use synchronous model. However, we have the upper bound on backoff counter, as in real-world applications.

\textbf{Message length}. Because protocols focus on conflict resolution, which is the main point behind the stability -- message length squeezed to some small constant value allows us to study protocols directly. Also real-applications message length can be seen as number of some unit-long messages combined into a single one, hence it can be viewed as a sort of channel-withholding mechanism unrelated to conflict resolution and universal for different protocols.

\textbf{Termination of undelivered messages}. \algoname{Backoff} protocol terminates undelivered messages after some timeout. We do not use such a mechanism in order to have correct evaluation for destabilization points of protocols. For rates lower than critical the mechanism clears the system from obsolete packets, thus lack of it does not seriously affect the workflow. For rates higher than critical it can hide protocols inability to transmit the same amount of packets as have been injected what is the case of our study.

\textbf{Synchronous model}. Real world applications are asynchronous, that is they function in real time. Still they are using clocks, what makes everything to be slotted in terms of clock ticks. \algoname{Backoff} algorithm uses time windows (defined by number of those clock rounds) for its transmission activity. In our synchronous model we make those clock rounds bigger so that transmission phase is the number of ticks needed to transmit a message and listening phase is amount of time needed to detect collision.

\section{Boundaries for system size $n = 32$}
\label{appendix:n32}
Protocols ave-max queues against injection rates $\rho \in \left[0,1\right]$ with a step of $0.001$ for a system size $n=32$ are put to a single plot to compare {\it (Figure \ref{QbyRo})}.
\begin{figure}[h]
\includegraphics[width=90mm,height=50mm]{../figures/ro_q_a2_1.png}
  \caption{Ave-max queue size by injection rates. 12 O'clock Adaptive (green), Full-sensing (orange) and Backoff polynomial (purple), square polynomial (red), exponential (blue), 8-light Interleaved-Selections (gray), Round-Robin (black) protocols for system size $32$ against injection rates $\rho \in \left[0,1\right]$ after 1 mln rounds.}
  \label{QbyRo}
\end{figure}

\algonamebf{Acknowledgement-based} protocols destabilize first, with \algoname{Round-Robin} queues size blowing for injection rates close to $\rho = 0.1$ and $\rho=0.31$ for 8-light \algoname{Interleaved-Selectors}. However note that those algorithms are literally tapes with binary information to-transmit or not to-transmit what makes them the most hardware-tolerant algorithms.

\textbf{\algonamebf{Backoff} polynomial} protocols destabilize at rates close to $\rho=0.4$ and $\rho=0.45$ accordingly. It can be described as too slow, in comparison to injection rates, adoption of the timeout window. After this critical point the protocol shows linear dependency of the queue size to injection rates.

\textbf{\algonamebf{Backoff} exponential} protocol stability boundary is more difficult to be defined in the scope of 1 mln rounds of the current study -- it has no clear destabilization point, but shows comparably fast to stable protocols queue growth around injection rates $\rho = 0.35$.

\algonamebf{12 O'clock} protocols show relatively rapid queue growth for injection rates around $\rho=0.1$ which can be described as movement from \algoname{Round-Robin} behaviour to \algoname{Move-Big-To-Front} one. Note that pure \algoname{Round-Robin} algorithm destabilizes on those rates. Full-sensing version of the \algoname{12 O'clock} destabilizing for rates around $\rho=0.969$ which is coherent with its theoretical limit for this system size: $\rho = \frac{31}{32} = 0.96875$.

\section{Additional simulations}
\subsection{Stability by system size}
In general all of the protocols but \algoname{12 O'clock} destabilize at some point, and because of the scale of destabilization charts show rather how protocol destabilize, than how their queues behave with stable injection rates. For this case we can describe the darker flat space as the stable one. For a case of \algoname{Backoff} protocols you may see that stability border is not always well defined {\it (Figure \ref{RRQ})}.

\subsection{The impact of different packet distribution on queues}
Because of the focused adversary nature, we may observe the impact of different packet distribution on queue size - for small system sizes its much closer to be flat than in big systems, where its definitely not flat.

The nature of the phenomenon is nicely illustrated by the \algoname{Round-Robin} which is known to have small queues in case of equal packet distribution {\it (Figure \ref{BEQ})}. 

\subsection{Acknowledgement-based algorithm observations}
The \algoname{Interleaved-Selectors} algorithm uses \algoname{Round-Robin} as one of the selectors and in case if no suitable 8-light $(n, \omega)$ could be generated - the only selector. As you may observe on {\it (Figure \ref{ISQ})} for a system size up to 16 it bases itself only on \algoname{Round-Robin} algorithm. For bigger systems the pattern changes, as more efficient selectors against focused injection appear within the algorithm. The irregular character of the queue behavior is explained by independent selector generation for each of the system size.

\begin{figure}
\includegraphics[width=90mm,height=90mm]{../figures/3d_ad.png}
\caption{12 O'clock Adaptive ave-max queue size by injection rates and system size.}
\end{figure}

\begin{figure}
\includegraphics[width=90mm,height=90mm]{../figures/3d_fs.png}
\caption{12 O'clock Full-sensing ave-max queue size by injection rates and system size.}
\end{figure}

\begin{figure}
\includegraphics[width=90mm,height=90mm]{../figures/3d_ac1.png}
\caption{Round-Robin ave-max queue size by injection rates and system size.}
\label{RRQ}
\end{figure}

\begin{figure}
\includegraphics[width=90mm,height=90mm]{../figures/3d_ac8.png}
\caption{8-light Interleaved Selectors ave-max queue size by injection rates and system size.}
\label{ISQ}
\end{figure}

\begin{figure}
\includegraphics[width=90mm,height=90mm]{../figures/3d_be.png}
\caption{Backoff exponential  ave-max queue size by injection rates and system size.}
\label{BEQ}
\end{figure}

\begin{figure}
\includegraphics[width=90mm,height=90mm]{../figures/3d_bs.png}
\caption{Backoff square  ave-max queue size by injection rates and system size.}
\end{figure}

\begin{figure}
\includegraphics[width=90mm,height=90mm]{../figures/3d_bl.png}
\caption{Backoff linear  ave-max queue size by injection rates and system size.}
\end{figure}

\begin{figure}
\includegraphics[width=90mm,height=90mm]{../figures/3d_fs_e.png}
\caption{12 O'clock Full-sensing  average energy usage by injection rates and system size.}
\end{figure}

\begin{figure}
\includegraphics[width=90mm,height=90mm]{../figures/3d_be-e.png}
\caption{Backoff exponential average energy usage by injection rates and system size.}
\end{figure}

\begin{figure}
\includegraphics[width=90mm,height=90mm]{../figures/3d_bs-e.png}
\caption{Backoff square average energy usage by injection rates and system size.}
\end{figure}

\begin{figure}
\includegraphics[width=90mm,height=90mm]{../figures/3d_bl-e.png}
\caption{Backoff linear average energy usage by injection rates and system size.}
\end{figure}
